# Supplementary material for: Uncovering the Deep Filter Bubble: Narrow Exposure in Short-Video Recommendation
Source: arXiv:2403.04511 source file (2024-03-07)
Supplement: Supplementary file 1 [file 6.appendix.tex]

\section{APPENDIX}

\subsection{Datasets}\label{app::dataset}
We use two datasets to conduct experiments, including a public e-commerce dataset and an industrial short-video dataset, which are also adopted by the SOTA sequential recommendation model, SURGE \cite{chang2021sequential}.
Both of them are in million scale and collected from real-world applications.
% Basic statistics of the two datasets are summarized in Table \ref{tab::dataset}, where Average Length indicates the average length of user interaction sequences.
% \begin{itemize}[leftmargin=*]
% 	\item \textbf{Taobao\footnote{\url{https://tianchi.aliyun.com/dataset/dataDetail?dataId=649}}.} We use the click-behavior data from Nov. 25th to Dec. 3rd, 2017. We adopt 10-core settings \cite{he2017neural} to filter out inactive entities. To evaluate the recommendation performance, we use all the instances till Dec. 1st as training data, the instances on Dec. 2nd for validation, and evaluate the final performance with the instances on Dec. 3rd.
% 	\item \textbf{Kuaishou\footnote{\url{https://www.kuaishou.com}}.} This industrial dataset is collected from Kuaishou, one of the largest short-video platforms in China. We extract the behavioral logs from Oct. 22nd to 28th, 2020. We use the click-behavior data and also adopt 10-core settings. We keep the instances of the first six days as the training set and reserve the last day for validation (before 12 pm) and test (after 12 pm).
% \end{itemize}
% We adopt two large-scale datasets, and both are collected from real-world applications.
The details of the adopted datasets are introduced as follows,
\begin{itemize}[leftmargin=*]
	\item \textbf{Taobao}\footnote{\url{https://tianchi.aliyun.com/dataset/dataDetail?dataId=649}}. This dataset \cite{zhu2018learning} is collected from the largest e-commerce platform in China, and it is widely used as a benchmark dataset for recommendation research \cite{zhu2018learning, zhu2019joint, pi2019practice}. It contains the user behaviors, including click, cart, and purchase from November 25 to December 3, 2017. We use the click data and adopt 10-core settings to filter out inactive entities. To evaluate the recommendation performance, we use all the instances till December 1 as training data. We use the instances on December 2 for validation and evaluate the final performance with the instances on December 3.
	\item \textbf{Kuaishou\footnote{\url{https://www.kuaishou.com}}.} This industrial dataset is collected from Kuaishou APP, one of the largest short-video platforms in China. Users can browse short videos uploaded by other users. We extract a subset of the logs from October 22 to October 28, 2020. The dataset contains user interactions with short videos, including click, like, follow (subscribe), and forward. We use the click data and also adopt 10-core settings to guarantee data quality. We keep the instances of the first 6 days as training set, and reserve the last day for validation (before 12 pm) and test (after 12 pm).
\end{itemize}
Table \ref{tab::dataset_appendix} shows the statistics of the two datasets after splitting.

\subsection{Baselines}\label{app::baseline}
We compare the proposed approach with the following competitive recommenders:
\begin{itemize}[leftmargin=*]
    \item \textbf{NCF} \cite{he2017neural}: This method is the state-of-the-art general recommender which combines matrix factorization and multi-layer perceptrons to capture the non-linearity of user interactions.
	\item \textbf{DIN} \cite{zhou2018deep}: This method uses attention mechanism to aggregate the historical interaction sequences. Attention weights are computed according to the target item.
	\item \textbf{LightGCN} \cite{he2020lightgcn}: This method is the state-of-the-art GCN based recommender and it utilizes neighborhood aggregation to capture the collaborative filtering effect.
	\item \textbf{Caser} \cite{tang2018personalized}: This method regards the sequence of items as images and extract sequential patterns with a convolutional network.
	\item \textbf{GRU4REC}~\cite{hidasi2015session}: This is the first approach that applies RNN to session-based recommendation system, with modified mini-batch training and ranking loss. 
	\item \textbf{DIEN} \cite{zhou2019deep}: This method improves DIN by combining attention with GRU to model the sequential pattern of user interests, and takes interests evolution into consideration.  
	\item \textbf{SASRec} \cite{kang2018self}: This method is the state-of-the-art sequential recommendation model which utilizes self-attention to capture sequential preferences.
	\item \textbf{SURGE} \cite{chang2021sequential}: This is the state-of-the-art recommendation approach which utilizes graph convolutional networks (GCN) to model user interest from sequential interactions.
	\item \textbf{SLi-Rec} \cite{yu2019adaptive}: This is the state-of-the-art algorithm which captures long-term interests with asymmetric-SVD and models short-term interests with a modified LSTM.
\end{itemize}

\begin{table}[t!]
    \caption{Statistics of the datasets.}
    \label{tab::dataset_appendix}
    \begin{tabular}{cccc}
      \toprule
      dataset & train & validation & test \\
      \midrule
      Taobao & 1,094,775 & 191,946 & 184,434 \\
      Kuaishou & 12,925,390 & 641,580 & 1,385,689 \\
      \bottomrule
    \end{tabular}
\end{table}

\subsection{Implementation Details}\label{app::implementation}
We implement all the models with the Microsoft Recommenders framework \cite{argyriou2020microsoft} based on TensorFlow \cite{abadi2016tensorflow}. We use the Adam optimizer \cite{kingma2014adam}.
Embedding size $d$ is set as 40.
We use a two-layer MLP with hidden size [100, 64] for interaction estimation.
Batch normalization is enabled for the MLP, and the activation function is ReLU.
The maximum length for user interaction sequences is 50 for Taobao dataset and 250 for Kuaishou dataset.
We use grid-search to find the best hyper-parameters.
The optimal settings for our proposed implementation are: $L_2$ regularization weight is 1e-6. Batchsize is 500. Learning rate is 0.001. $\beta$ is 0.1. $l_t$ is 5 for Taobao dataset and 10 for Kuaishou dataset. $k$ is 3 for Taobao dataset and 5 for Kuaishou dataset. $\mathcal{L}_{\text{con}}$ is $\mathcal{L}_{\text{tri}}$ for Taobao dataset and $\mathcal{L}_{\text{bpr}}$ for Kuaishou dataset.

\subsection{More Studies on the Proposed Method}\label{app::ablation}

\begin{table}[t]
    \caption{Performance of different $k$ on Taobao dataset.}
    \label{tab::taobao_k}
    \begin{tabular}{c|cccc}
      \toprule
      $k$ & AUC & GAUC & MRR & NDCG@2 \\
      \midrule
      1 & 0.8975 & 0.8927 & 0.4306 & 0.3717 \\
      2 & 0.8956 & 0.8938 & 0.4364 & 0.3798 \\
      3 & 0.8953 & 0.8936 & 0.4372 & 0.3788 \\
      4 & 0.8936 & 0.8924 & 0.4331 & 0.3747 \\
      \bottomrule
    \end{tabular}
\end{table}

In this section, we conduct experiments to investigate how the proposed method performs under different values of several introduced hyper-parameters. We also include further ablation studies on several components.

\noindent\textbf{Short-term Proxy $k$.}
In the proposed method, we use mean pooling of the recent $k$ interacted items as the proxy representation for short-term interests.
Table \ref{tab::taobao_k} illustrates the results of different $k$ on Taobao dataset.
We can observe that setting $k$ as 1 achieves poorer performance except for AUC, which means only using the last interacted item as proxy for short-term interests is not a good choice since one interaction can be noise with large possibilities.

\noindent\textbf{Interests Evolution}
Short-term interests are quite different from long-term interests with respect to their dynamics over time, thus we utilize a GRU to generate query vectors in Eqn (\ref{eq::short}) which simulates the evolution of short-term interests.
We study the effect of interests evolution and results are shown in Table \ref{tab::evolution}.
% conduct experiments to compare the performance of using simple embedding tables without interests evolution.
% Table \ref{tab::evolution} shows the results.
We can observe that removing interests evolution causes a significant decrease of accuracy on both datasets, which confirms the necessity of modeling different semantics of LS-term interests.
%Although we only use a simple GRU model, the performance gap indicates that simulating the process of interests evolution is indeed helpful to improve the performance of recommendation.
%We believe that using more advanced models such as Transformers \cite{vaswani2017attention} would achieve even better performance and leave it for future work.

\begin{table}
\small
	\caption{Study of interests evolution.}
	\vspace{-10px}
	\label{tab::evolution}
	\begin{tabular}{c|c|ccccc}
    \toprule
    Dataset & Evolution & AUC & GAUC & MRR & NDCG@2 \\ 
    \midrule
    \multicolumn{1}{c|}{\multirow {2}{*}{Taobao}} & yes & 0.8953 & 0.8936 & 0.4372 & 0.3788 \\
    \multicolumn{1}{c|}{} & no & 0.8847 & 0.8884 & 0.4320 & 0.3735 \\
    \hline
    \multicolumn{1}{c|}{\multirow {2}{*}{Kuaishou}} & yes & 0.8563 & 0.8718 & 0.9382 & 0.9544 \\
    \multicolumn{1}{c|}{} & no & 0.8202 & 0.8333 & 0.9226 & 0.9429 \\
    \bottomrule
    \end{tabular}
    % \vspace{-10px}
\end{table}

\noindent\textbf{Study of Different Design Choices}
We further compare different design choices in CLSR.
%Specifically, we investigate different options for short-term interests encoder $\rho$ and contrastive loss function $\mathcal{L}_\text{con}$ in Eqn (\ref{eq::rho}) and (\ref{eq::L_con}).
Specifically, we investigate different options for short-term interests encoder and contrastive loss function in Eqn (\ref{eq::rho}) and (\ref{eq::L_con}).
For the RNN $\rho$ in the short-term interests encoder $\psi$, we compare LSTM \cite{hochreiter1997long}, GRU \cite{chung2014empirical}, and Time4LSTM proposed by SLi-Rec \cite{yu2019adaptive}.
For $\mathcal{L}_\text{con}$, we compare BPR loss and triplet loss.
Table \ref{tab::design} shows the results of different design choices.
We can observe that Time4LSTM outperforms LSTM and GRU on both datasets, indicating that the time interval feature is helpful for LS-term interests modeling, which is ignored by LSTM and GRU.
% as the other two encoders ignore the time interval features.
As for contrastive loss, each loss function fails to consistently outperform the competitor, which can be explained by the different scales of the two datasets.
In fact, CLSR is a highly general framework in which many sequential encoders and loss functions can be utilized. 
We leave the further study as future work.

\begin{table}
\small
	\caption{Comparison of different design choices.}
	\vspace{-10px}
	\label{tab::design}
	\begin{tabular}{c|ccc|cc}
    \toprule
    Dataset & LSTM & GRU & Time4LSTM & BPR & Triplet \\ 
    \midrule
    Taobao & 0.8872 & 0.8860 & \bf{0.8953} & 0.8909 & \bf{0.8953} \\
    Kuaishou & 0.8240 & 0.8259 & \bf{0.8563} & \bf{0.8563} & 0.8102\\
    \bottomrule
    \end{tabular}
    \vspace{-10px}
\end{table}

\noindent\textbf{Fusion Predictor GRU.}
In the proposed adaptive fusion model based on the attention technique, we incorporate both the target item and the historical sequence to predict whether the next interaction is driven by long or short-term interests.
Specifically, we adopt a separate GRU that takes the historical sequence as input, and we use the final state as the input of MLP.
We conduct experiments to investigate whether taking the historical sequence into consideration is necessary.
Table \ref{tab::fusion_gru} illustrates the results of the proposed method with and without the fusion predictor GRU.
We can observe that removing the fusion predictor GRU makes the recommendation performance drop significantly, which confirms that the importance of long or short-term interests is largely determined by the historical sequence.

\begin{table}[t]
	\caption{Study of fusion predictor GRU on Taobao dataset.}
	\label{tab::fusion_gru}
	\begin{tabular}{c|ccccc}
    \toprule
    Method & AUC & GAUC & MRR & NDCG@2 \\ 
    \midrule
    w/ GRU & 0.8953 & 0.8936 & 0.4372 & 0.3788 \\
    w/o GRU & 0.8817 & 0.8853 & 0.4275 & 0.3692 \\
    \bottomrule
    \end{tabular}
\end{table}

\noindent\textbf{Attentive Encoder}
As introduced in Equation (\ref{eq::att1}), the proposed attentive encoder adopts a MLP to compute attention weights.
The inputs of the MLP are composed of the key vector, query vector, the element-wise difference, and multiplication of key and query.
We compare the MLP based attention with simple inner product based attention:
\begin{equation}
    \alpha_k'= \langle\bm{v_k}, \bm{u_l}\rangle.
\end{equation}
Table \ref{tab::attention} illustrates the comparison of MLP and inner product based attention.
Results in Table \ref{tab::attention} show that MLP based attention outperforms inner product-based attention with a significant margin, which indicates that the relation between user interests and historical sequences is non-linear and can not be well captured by linear operators like the inner product.

\begin{table}[t]
	\caption{Study of attentive encoder on Taobao dataset.}
	\label{tab::attention}
	\begin{tabular}{c|ccccc}
    \toprule
    Attention & AUC & GAUC & MRR & NDCG@2 \\ 
    \midrule
    MLP & 0.8953 & 0.8936 & 0.4372 & 0.3788 \\
    Inner Product & 0.8684 & 0.8706 & 0.4051 & 0.3480 \\
    \bottomrule
    \end{tabular}
\end{table}
\noindent\textbf{Discrepancy Supervision}
In our proposed method, we do not add an extra discrepancy loss on the LS-term interests to make them independent with each other as other works \cite{wang2020disentangled,zheng2021disentangling}, since we believe self-supervision is enough to accomplish disentanglement.
During our experiments, we tried to add an independent loss between the two interests as, and AUC drops by 0.01, which verifies our point.
It is worthwhile to notice that many existing works \cite{ma2020disentangled,cen2020controllable,wang2020disenhan} also did not use the independent loss.

\noindent\textbf{More Counterfactual Evaluations}
\begin{figure}[t]
  \centering
  \includegraphics[width=\linewidth]{figs/truncate_kuaishou.eps}
  \vspace{-15px}
  \caption{Counterfactual (truncate) evaluation of the proposed method on Kuaisohu dataset.}
  \Description{Counterfactual (truncate) evaluation of the proposed method on Kuaisohu dataset.}
  \label{fig::truncate_kuaishou}
%   \vspace{-15px}
\end{figure}
% Due to space limit, we only demonstrate the results of the counterfactual evaluation under truncate protocol on Taobao dataset.
% Here we show the results on Kuaishou dataset.
Figure \ref{fig::truncate_kuaishou} illustrates the AUC of click and like on Kuaishou dataset with available history length $k$ varying from 50 to 250.
Results on Kuaishou dataset are in line with results on Taobao dataset in Figure \ref{fig::truncate}(a).
Specifically, AUC of like is more sensitive to the length of available history and improves drastically as $k$ increases, while AUC of click does not improve much as we increase $k$.
Since like reflects more about the user's long-term interest, it is necessary to have access to the entire user interaction sequence.
Meanwhile, click is more about short-term interest, and thus it can be largely captured from the recent history, and looking back to early history will not bring further gains.

\noindent\textbf{Complexity.}
We use a single GPU to compare the complexity.
The training time of CLSR and typical baselines on Taobao dataset are shown in Table \ref{tab::complexity}.
The parameter scale of CLSR is comparable with SLi-Rec (both takes 4.1Gb GPU memory).

\begin{table}[t!]
	\caption{Training time cost on Taobao dataset.}
	\label{tab::complexity}
	\begin{tabular}{c|ccc}
    \toprule
    Method & GRU4REC & SLi-Rec & CLSR \\ 
    \hline
    Time &  27.8min & 26.7min & 28.2min \\
    \bottomrule
    \end{tabular}
\end{table}
